# Supplementary material for: Human-Aligned Skill Discovery: Balancing Behaviour Exploration and Alignment
Source: arXiv:2501.17431 source file (2025-01-29)
Supplement: Supplementary file 1 [file hazard_room.tex]

\subsubsection{Full Qualitative Results}
