# Supplementary material for: Human-Aligned Skill Discovery: Balancing Behaviour Exploration and Alignment
Source: arXiv:2501.17431 source file (2025-01-29)
Supplement: Supplementary file 2 [file push_room.tex]

\subsubsection{Push Room}
